# Supplementary material for: Dynamical Optimal Transport on Discrete Surfaces
Source: arXiv:1809.07083 source file (2018-09-19)
Supplement: Supplementary file 1 [file section_appendix.tex]

\appendix 

\hugo{Just storage for the moment}

Proof of the proposition about the inf sup exchange 

\begin{proof}
We will write only a formal $\inf-\sup$ exchange; a more formal proof requires the use of Rockefeller-Fenchel duality \cite[Theorem 1.9]{Villani2003}. We start with \eqref{equation_BB_discrete_dual} and introduce a Lagrange multiplier $\mu : [0,1] \times V \to \R_+$: 
\begin{multline}
W_d^2(\bar{\mu}^0, \bar{\mu}^1) = \sup_{\varphi} \inf_{\mu}  \sum_{v \in V} \varphi^1_v \bar{\mu}^1_v - \sum_{v \in V} \varphi^0_v \bar{\mu}^0_v \\ - \int_0^1 \left( \sum_{v \in V} |v| \mu^s_v \left( \dr_s \varphi^s_v + \displaystyle{ \frac{1}{2} \frac{\sum_{t \ : \  v \in t  } |t| \| (G \varphi)^s_t \|^2 }{  3 |v|}}  \right) \right) \dint s
\end{multline}
Rearranging the last sum so that it is indexed by triangles and using the identity $- \| (G \varphi)_t \|^2 = \inf_{\vbf} [- \vbf \cdot (G \varphi)_t + \frac{1}{2} \| \vbf \|^2]$, we see that 
\begin{multline}
W_d^2(\bar{\mu}^0, \bar{\mu}^1) = \sup_{\varphi} \inf_{\mu, \vbf} \sum_{v \in V} \varphi^1_v \bar{\mu}^1_v - \sum_{v \in V}  \varphi^0_v \bar{\mu}^0_v \\ 
- \int_0^1 \left( \sum_{v \in V} |v| \mu^s_v  \dr_s \varphi^s_v \right) \dint s \\ 
+ \int_0^1 \left( \sum_{t \in T} |t| \underbrace{\left( \frac{1}{3} \sum_{v \in V \text{ s.t. } v \in t} \mu^s_v  \right)}_{\hat{\mu}^s_t} \left( - \vbf^s_t \cdot (G \varphi)^s_t + \frac{1}{2} \| \vbf^s_t \|^2 \right) \right) \dint s.
\end{multline}
Once the $\inf$ and the $\sup$ are exchanged, taking the supremum in $\varphi$ yields a weak formulation of the discrete continuity equation with the boundary conditions $\bar{\mu}^0, \bar{\mu}^1$. In particular, it implies that the mass is conserved, and hence $\mu$ is valued in $\P(S)$. The remaining term is nothing that the integral over time of the kinetic energy. 
\end{proof} 

Definition of the augmented Lagrangian 

In the end, the Lagrangian can be written 
\begin{multline}
\label{equation_discrete_Lagrangian}
L(\varphi,A,B,\mu,m) \eqdef  \sum_{v \in V} |v| \varphi^1_v \bar{\mu}^1_v - \sum_{v \in V} |v| \varphi^0_v \bar{\mu}^0_v \\ 
+ \sum_{(s,v) \in \Gtimec V} \Delta s |v| \mu^s_v \left( A_v^s - (\Delta\varphi)^s_v \right) \\
+ \sum_{ (s,i,t,v) \in \Gtimec \times \{\pm 1\} \times T \times V } \Delta s |t| m^{s,i}_{t,v} \cdot \left(  B^{s,i}_{t,v} - (G\varphi)_t^{s + i \Delta s / 2} \right)  \\
- \frac{r}{2} \Big[  \sum_{(s,v) \in \Gtimec V} \Delta s |v| \left( A_v^s - (\Delta \varphi)^s_v \right)^2 \\
+ \sum_{ (s,i,t,v) \in \Gtimec \times \{\pm 1\} \times T \times V } \Delta s |t| \|  B^{s,i}_{t,v} - (G\varphi)_t^{s + i \Delta s / 2} \|^2
\Big],
\end{multline}
and the variables $A,B$ are subject to the constraints 
\begin{equation}
\label{equation_constraint_AB}
A^s_v + \displaystyle{ \frac{1}{2} \sum_{i \in \{-1,1\}} \frac{1}{2} \frac{\sum_{t \ : \  v \in t  } |t| \| B^{s,i}_{v,t} \|^2 }{  3 |v|}}   \leqslant 0
\end{equation}
for all $(s,v) \in \Gtimec \times V$.
